# Supplementary material for: Observation of Flat Frequency Bands at Open Edges and Antiphase Boundary Seams in Topological Mechanical Metamaterials
Source: arXiv:2005.06450 ancillary file (2020-11-24)
Supplement: Supplementary file 1 [file Supplemental-Text.pdf]

# Supplemental Material for "Observation of Flat Frequency Bands at Open Edges and Antiphase Boundary Seams in Topological Mechanical Metamaterials"

Kai Qian,<sup>1</sup> Linghua Zhu,<sup>2</sup> Keun Hyuk Ahn,<sup>1</sup> and Camelia Prodan<sup>1</sup>

<sup>1</sup>*Department of Physics, New Jersey Institute of Technology, Newark, New Jersey, USA*

<sup>2</sup>*Department of Physics, Virginia Tech, Blacksburg, Virginia, USA*

## I. THEORETICAL ANALYSIS

In this section, further details of the theoretical analysis are provided. As described in Ref. [S1], the normalized Lagrangian for two magnetically coupled spinners is approximately given by

$$\frac{L(\varphi_1, \varphi_2, \dot{\varphi}_1, \dot{\varphi}_2)}{2\pi^2 I} = \frac{1}{4\pi^2} \dot{\varphi}_1^2 + \frac{1}{4\pi^2} \dot{\varphi}_2^2 - \frac{1}{2} \alpha (\varphi_1^2 + \varphi_2^2) - \beta \varphi_1 \varphi_2, \quad (\text{S1})$$

where  $I$  represents the moment of inertia of each spinner,  $\varphi_1$  and  $\varphi_2$  the rotation angles of the two spinners from the equilibrium states. The parameters  $\alpha$  and  $\beta$  represent the coefficients in potential energy terms and depend on the strengths of the magnets attached at the end of spinner arms and the distance between the magnets. If we represent the parameter  $\beta$  for the spinner pairs connected by the blue, red, and green lines in Fig. 1(b) in the main text as  $\beta_b$ ,  $\beta_r$ , and  $\beta_g$ , the condition for the gap opening is  $\beta_g < (\beta_b + \beta_r)/2$ , under which the system becomes topological if  $\beta_b < \beta_r$  and nontopological if  $\beta_b > \beta_r$ . For the topological insulator spinner systems, the parameter values are  $\beta_b = 106.7 \text{ Hz}^2$ ,  $\beta_r = 280.0 \text{ Hz}^2$ , and  $\beta_g = 83.4 \text{ Hz}^2$ .

Applying periodic boundary conditions in the  $n_2$  direction, the localization length  $\xi(k_2)$  for the edge states with the wave vector  $k_2$  is found to be

$$\xi(k_2) = \frac{4}{\ln \frac{\beta_r^2 + \beta_g^2 + 2\beta_r\beta_g \cos k_2}{\beta_b^2 + \beta_g^2 + 2\beta_b\beta_g \cos k_2}}, \quad (\text{S2})$$

similar to the localization length for the 1D SSH system [S2]. The amplitude of the oscillation for the left-edge state with the wave vector  $k_2$  decays as

$$A_{k_2}(n_1, n_2) = \begin{cases} Ae^{-(n_1-1)/\xi(k_2)} & \text{for odd } n_1 \\ 0 & \text{for even } n_1 \end{cases} \quad (\text{S3})$$

and for the right-edge state as

$$B_{k_2}(n_1, n_2) = \begin{cases} 0 & \text{for odd } n_1 \\ Be^{-(N_1-n_1)/\xi(k_2)} & \text{for even } n_1 \end{cases} \quad (\text{S4})$$

in the limit of the large edge-to-edge distance,  $N_1$ . With the parameter values given above for the topological spinner systems, we obtain the localization length  $\xi(k_2)$  versus  $k_2$  as shown in Fig. S1, with  $\xi(k_2)$  ranging between 0.9 at  $k_2 = \pm\pi$  and 3.1 at  $k_2 = 0$  in the unit of the

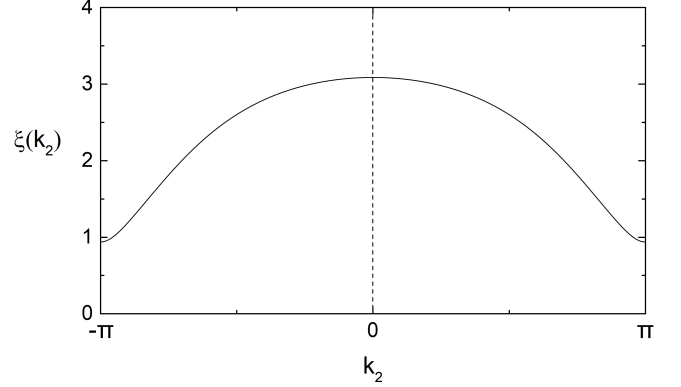

FIG. S1. Localization length  $\xi(k_2)$  versus the edge state wave vector  $k_2$  in the limit of the large edge-to-edge distance  $N_1$  for the topological spinner systems.  $\xi(k_2)$  varies between 0.9 at  $k_2 = \pm\pi$  and 3.1 at  $k_2 = 0$ .

spinner-to-spinner distance. The above theoretical results are used to analyze the experimental results shown in Figs. 4(e) and 4(f) in the main text.

The frequency splitting  $\Delta f(k_2)$  between the two edge modes with the wave vector  $k_2$  is  $\Delta f(k_2) = CN_1 e^{-N_1/\xi(k_2)}$  in the limit of large  $N_1/\xi(k_2)$ . Since the localization length  $\xi(k_2)$  is largest at  $k_2 = 0$ , the edge band width  $\Delta f_0$  is given by

$$\Delta f_0 = CN_1 e^{-N_1/\xi_0} \quad (\text{S5})$$

in the limit of large  $N_1/\xi_0$ , where  $\xi_0 = \xi(k_2 = 0)$ , the localization length at  $k_2 = 0$ . The plot of  $\ln(\Delta f_0)$  versus  $N_1$  for experimental data is fitted into  $\ln(\Delta f_0) = \ln C + \ln N_1 - N_1/\xi_0$  to estimate  $\xi_0$ , as shown in Fig. 2(l) in the main text.

## II. ADEQUACY OF THE CHOSEN SPINNER SYSTEM SIZES

In this section, the sizes experimentally chosen for the spinner systems are shown to be adequate to demonstrate the flatness of the edge bands. Since Fig. 2(k) in the main text demonstrates that experimental results agree well with numerical simulations for the edge band width, numerical simulations with open boundary conditions are used for the analysis.

First, for the  $N_1 \times N_2$  spinner system, we fix  $N_1$  to 4, 6, 8, 10, and 12, the values chosen for the experiments,

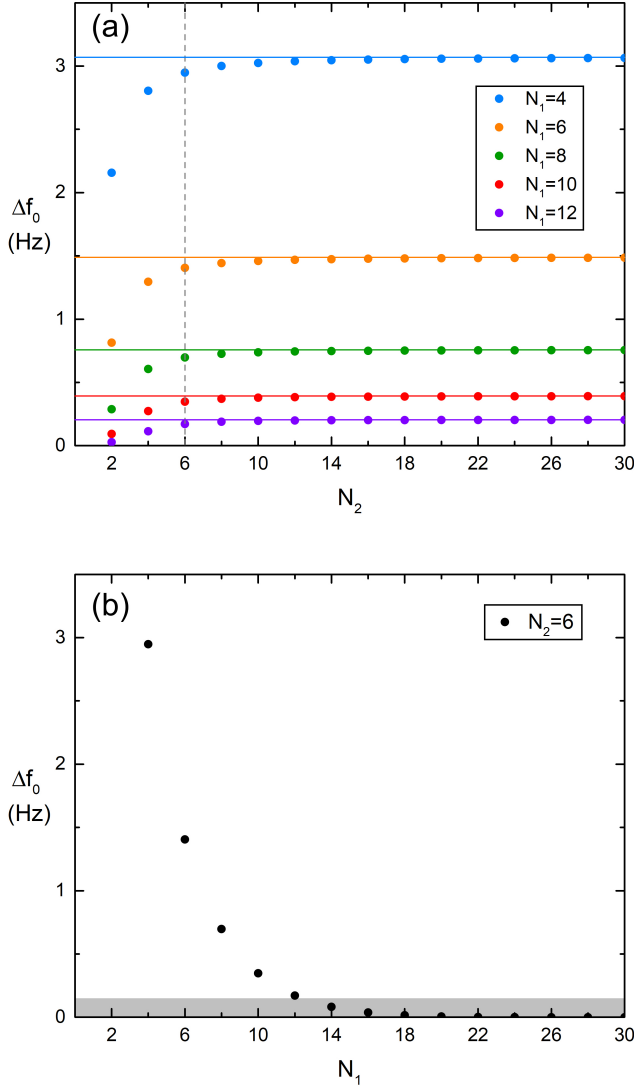

FIG. S2. (a) Symbols: Edge band width  $\Delta f_0$  versus  $N_2$ , calculated for  $N_1 \times N_2$  systems with  $N_1 = 4, 6, 8, 10$ , and  $12$  and open boundary conditions. Horizontal solid lines:  $\Delta f_0$  calculated for  $N_2 = 1,000$  as a large  $N_2$  limit for each case of  $N_1$ . Vertical dashed line:  $N_2 = 6$  chosen for experimental setups. (b) Edge band width  $\Delta f_0$  versus  $N_1$ , calculated for the  $N_1 \times 6$  systems with open boundary conditions. The gray area approximately represents the experimental resolution, below which the edge band width cannot be measured reliably.

and varies  $N_2$  up to 1,000 to see how the edge band width  $\Delta f_0$  depends on  $N_2$ . The results in Fig. S2(a) show that the edge band width  $\Delta f_0$  increases as  $N_2$  increases. The values of  $\Delta f_0$  at  $N_2 = 1,000$ , which could be considered as the large  $N_2$  limit, are shown as horizontal lines. The results show that the edge band widths  $\Delta f_0$  at  $N_2 = 6$  (vertical dashed line), the size chosen for experimental setups for the results in Fig. 2 in the main text, are only about  $0.12 \sim 0.03$  Hz, or  $5 \sim 15\%$  smaller than the corresponding large  $N_2$  limits for the systems with  $N_1 = 4, 6, 8, 10$ , and  $12$ , which indicates that the choice  $N_2 = 6$  is adequate. Relatively quick saturation of  $\Delta f_0$  for  $N_2$  as small as 6 in Fig. S2(a) is consistent with the edge band width being determined at  $k_2 = 0$  [See Eq. (S5)], which is insensitive to the number of  $k_2$ -points.

Next, with  $N_2$  fixed at 6, we examine how adequate the experimental choice of  $N_1 = 4, 6, 8, 10, 12$  is to represent the trend in the edge band width  $\Delta f_0$  versus  $N_1$ . The results in Fig. S2(b) show that the edge band width  $\Delta f_0$  continues to decrease as the edge-to-edge distance  $N_1$  increases further up to 30, and becomes below the experimental resolution, shown in gray area, beyond around  $N_1 = 12$ . Rapid decrease of the edge band width with the increase in  $N_1$  from  $N_1 = 4$  to 12 reflects the relatively short localization length,  $\xi(k_2) = 0.9 \sim 3.1$  in the unit of spinner-to-spinner distance for the chosen experimental parameters. The experimental results for  $N_1 = 6, 8, 10$ , and  $12$  also allow us to reveal exponential decrease of the edge band width  $\Delta f_0$  with respect to  $N_1$ , consistent with the theoretical predictions, as shown in Fig. 2(l) in the main text. Therefore, our choice of  $N_1 = 4, 6, 8, 10, 12$  and  $N_2 = 6$  for experimental setups is adequate to show that the edge band would have a vanishing width and become flat in the whole projected reciprocal space in the limit of large edge-to-edge distance.

- 
- [S1] D. J. Apigo, K. Qian, C. Prodan, and E. Prodan, Topological edge modes by smart patterning, *Phys. Rev. Mater.* **2**, 124203 (2018).  
[S2] J. K. Asbóth, L. Oroszlány, and A. Pályi, *A Short Course on Topological Insulators: Band structure and edge states in one and two dimensions* (Springer, Cham, 2016).
